# Supplementary material for: Estimation with Norm Regularization
Source: arXiv:1505.02294 source file (2015-11-30)
Supplement: Supplementary file 1 [file supp_general_norms.tex]

\documentclass[bezier,amstex]{article} % For LaTeX2e
\usepackage{nips14submit_e,times}

\usepackage{times}
\usepackage{graphicx}
\usepackage[rflt]{floatflt}
\usepackage{epsfig,subfigure}
\usepackage{amsmath,amssymb,algorithm,algorithmic,theorem,float,bbm,bm,enumerate,multirow}
\usepackage{rotating}
\usepackage{array}

\usepackage[small,it]{caption}
\usepackage[small,compact]{titlesec}
\usepackage{times}
\usepackage{color}
\usepackage{url}

\usepackage{chngcntr}

\usepackage[numbers]{natbib}

\usepackage{nameref}
\usepackage{zref-xr}
\zxrsetup{toltxlabel}

\input{notation}

\newcommand{\ab}[1] {{\bf (Arindam Says: #1)}}

%\setcounter{footnote}{0}
%\sloppy
%
%\renewcommand{\theequation}{\thesection.\arabic{equation}}
%\newcommand{\newsection}{\setcounter{equation}{0}\section}
%
%\newtheorem{theorem}{Theorem}
%\newtheorem{proposition}[theorem]{Proposition}
%\newtheorem{lemma}[theorem]{Lemma}
%\newtheorem{corollary}[theorem]{Corollary}
%\newtheorem{definition}{Definition}
%\newtheorem{example}[theorem]{Example}
%\newtheorem{remark}[theorem]{Remark}

\title{Supplement: Estimation with Norm Regularization}

\author{
David S.~Hippocampus\thanks{ Use footnote for providing further information
about author (webpage, alternative address)---\emph{not} for acknowledging
funding agencies.} \\
Department of Computer Science\\
Cranberry-Lemon University\\
Pittsburgh, PA 15213 \\
\texttt{hippo@cs.cranberry-lemon.edu} \\
\And
Coauthor \\
Affiliation \\
Address \\
\texttt{email} \\
\AND
Coauthor \\
Affiliation \\
Address \\
\texttt{email} \\
\And
Coauthor \\
Affiliation \\
Address \\
\texttt{email} \\
\And
Coauthor \\
Affiliation \\
Address \\
\texttt{email} \\
(if needed)\\
}

% The \author macro works with any number of authors. There are two commands
% used to separate the names and addresses of multiple authors: \And and \AND.
%
% Using \And between authors leaves it to \LaTeX{} to determine where to break
% the lines. Using \AND forces a linebreak at that point. So, if \LaTeX{}
% puts 3 of 4 authors names on the first line, and the last on the second
% line, try using \AND instead of \And before the third author name.

%\nipsfinalcopy % Uncomment for camera-ready version

\zexternaldocument*{../main/nips_general_norms}
\zexternaldocument*{../main/main-conc}
\zexternaldocument*{../main/main-error}
\zexternaldocument*{../main/main-gauss-re}
\zexternaldocument*{../main/main-glm}
\zexternaldocument*{../main/main-intro}
\zexternaldocument*{../main/main-lambda}
\zexternaldocument*{../main/main-re}
\zexternaldocument*{../main/main-subgauss-re}
\zexternaldocument*{../main/nips_general_norms}

\begin{document}

%\counterwithout{equation}{section}

\maketitle

\section{Background and Preliminaries}
\input{back}

\section{Restricted Error Set and Recovery Guarantees}
\input{supp-error}

\section{Bounds on the Regularization Parameter}
\input{supp-lambda}

\section{Restricted Eigenvalue Conditions: Gaussian Designs}
\input{supp-gauss-re}

\section{Restricted Eigenvalue Conditions: Sub-Gaussian Designs}

\ab{Inactive section - borrow proofs to help the previous section in appendix.}

\subsection{Dependent Isotropic Sub-Gaussian Designs}
%\label{ssec:disg}
In this section, we consider the setting where the design matrix $\tilde{X}$ has isotropic sub-Gaussian rows, but the rows are dependent. In particular, we assume that $\vertiii{ \tilde{x}_{ij} }_{\psi_2} = k$,
and $E[\tilde{X_j} \tilde{X_j}^T] = \Gamma \in \R^{n \times n}$. We show that the gain condition holds for such dependent sub-Gaussian designs:

\textbf{Theorem \ref{thm:corrSubG}}
\textit{
Let $\tilde{X} \in \R^{n \times p}$ be a sub-Gaussian design matrix with isotropic rows and correlated columns with $E[\tilde{X}_j \tilde{X}_j^T] = \Gamma \in \R^{n \times n}$. Then, for any $A \subseteq S^{p-1}$ and any $\tau > 0$, with probability at least $(1- 2exp(-\eta_1 \tau^2) )$, we have
\beq
\inf_{u \in A} \| \tilde{X} u \|_2 \geq \sqrt{\tr(\Gamma)} -  \Lambda_{max}(\Gamma)~\eta_0 w(A)  - \tau~,
\eeq
where $\eta_0, \eta_1$ are constants which depend on the sub-Gaussian norm $\vertiii{ x_{ij} }_{\psi_2} = k$.}

\proof The analysis will use results from Lemma \ref{lem:disciig} and \ref{lem:ripdig}.

%\begin{lemm}
%Let $A \subseteq S^{p-1}$. Consider a symmetric matrix $B$ which satisfies, for some $\delta > 0$

%\beq
%\left | \|Bu\|_2^2 - Tr(\Gamma) \right | \leq \max(\delta, \delta^2)Tr(\Gamma), ~~ \forall u \in A
%\eeq

%Then,

%\beq
%\inf_{u \in A} \|Bu\|_2 \geq \sqrt{Tr(\Gamma)} - \delta \sqrt{Tr(\Gamma)}
%\eeq

%\label{lem:rip3}
%\end{lemm}

%\proof Let $z = \frac{\|Bu\|_2}{\sqrt{Tr(\Gamma)}}$. Therefore, using the elementary inequality

%\beq
%\max(|z - 1|, |z - 1|^2) \leq |z^2 - 1|
%\eeq

%we get,

%\beq
%\left | \frac{\|Bu\|_2}{\sqrt{Tr(\Gamma)}} - 1 \right | \leq \delta ~~ \Rightarrow \|Bu\|_2 \geq \sqrt{Tr(\Gamma)} - \delta \sqrt{Tr(\Gamma)}
%\eeq

%Taking infimum over all $u \in A$ gives the required result. \qed

With $B = \tilde{X}$ and following Lemma \ref{lem:ripdig}, it suffices to show that

\beq
\sup_{u \in A} \left | \|\tilde{X}u\|_2^2 - Tr(\Gamma) \right | \leq \max(\delta, \delta^2)Tr(\Gamma) \triangleq t, ~~ \forall u \in A
\eeq

where $\delta = \frac{\eta_0 w(A) \Lambda_{max}(\Gamma)}{\sqrt{Tr(\Gamma)}} + \frac{\tau}{\sqrt{Tr(\Gamma)}}$. From Lemma \ref{lem:disciig}, using a $\epsilon = \frac{1}{4}$-net $\cN_{\epsilon}(A)$ on $A \subseteq S^{p-1}$, we have

\beq
\begin{split}
\sup_{u \in A} \left | \|\tilde{X}u\|_2^2 - Tr(\Gamma) \right | = \sup_{u \in A} \left | \langle (\tilde{X}^T \tilde{X} - \I Tr(\Gamma))u, u \rangle \right | \leq 2 \max_{v \in \cN_{\epsilon}(A)} \left | \langle (\tilde{X}^T \tilde{X} - \I Tr(\Gamma))v, v \rangle \right | \\
= 2 \max_{v \in \cN_{\epsilon}(A)} \left | \|\tilde{X}v\|_2^2 - Tr(\Gamma) \right |
\end{split}
\eeq

As a result, it suffices to prove with high probability

\beq
\max_{v \in \cN_{\epsilon}(A)} \left | \|\tilde{X}v\|_2^2 - Tr(\Gamma) \right | \leq \frac{t}{2}
\eeq

Let $\tilde{Z} = \tilde{X}v$. Also $\tilde{X} = \Gamma^{1/2}X$ where $E[\tilde{X_j}\tilde{X_j}^T] = \Gamma$ and $X \in \R^{n \times p}$ has independent sub-Gaussian entries. Let $Z = Xv$ is an isotropic sub-Gaussian random vector, with each entry $Z_i = \langle X_i, v \rangle$ such that $\vertiii{Z_i}_{\psi_2} \leq K$. Then

\beq
\|\tilde{X}v\|_2^2 = \|\Gamma^{1/2}Z\|_2^2 = \|\sum_{j=1}^{n} Z_j \Gamma_j^{1/2} \|_2^2 = \sum_{j=1}^{n} Z_j^2 \|\Gamma_j^{1/2}\|_2^2 + \sum_{j,k \in [1,...,n], j \neq k} Z_j Z_k \langle \Gamma_j^{1/2}, \Gamma_k^{1/2} \rangle
\eeq

where $\Gamma_j^{1/2}, \Gamma_k^{1/2}$ denote the jth and kth columns of $\Gamma$ and $[1,...n]$ denotes a set containing the first n natural numbers. We assume that $\| \sum_{j=1}^{n} Z_j \Gamma_j^{1/2} \|_2^2 = Tr(\Gamma)$ almost surely. Then,

\beq
\|\tilde{X}v\|_2^2 =  \sum_{j=1}^{n} \|\Gamma_j^{1/2}\|_2^2 + \sum_{j,k \in [1,...,n], j \neq k} Z_j Z_k \langle \Gamma_j^{1/2}, \Gamma_k^{1/2} \rangle = Tr(\Gamma) + \sum_{j,k \in [1,...,n], j \neq k} Z_j Z_k \langle \Gamma_j^{1/2}, \Gamma_k^{1/2} \rangle
\eeq

Therefore, we get

\beq
| \|\tilde{X}v\|_2^2 - Tr(\Gamma)| \leq \left | \sum_{j,k \in [1,...,n], j \neq k} Z_j Z_k \langle \Gamma_j^{1/2}, \Gamma_k^{1/2} \rangle \right |
\eeq

The sum on the r.h.s is $\langle \Gamma_0 x,x \rangle$ where $\Gamma_0$ is the off-diagonal part of $\Gamma$. This can also be written as follows:

\beq
R_T(z) = \sum_{j \in T, k \in T^c} Z_j Z_k \langle \Gamma_j^{1/2}, \Gamma_k^{1/2} \rangle
\eeq

We state the following decoupling Lemma, the proof of which is provided on Pg. 38 of~\cite{vers12} to bound the above quantity

\begin{lemm}
Consider a double array of real numbers $(a_{ij})_{i,j = 1}^{n}$, such that $a_{ii} = 0$ for all $i$. Then

\beq
\sum_{i,j \in [1,...,n]} a_{ij} = 4 E \sum_{i \in T, j \in T^c} a_{i,j}
\eeq

where $T$ is a random subset of $[1,...,n]$ with average size $n/2$. In particular

\beq
4 \min\limits_{T \subseteq [1,...,n]} \sum_{i \in T, j \in T^c} a_{ij} \leq \sum_{i,j \in [1,...,n]} a_{ij} \leq 4 \max\limits_{T \subseteq [1,...,n]} \sum_{i \in T, j \in T^c} a_{ij}
\eeq
where the minimum and maximum are over all subsets of $[1,...,n]$. \qed
\label{lem:DecouplingLem}
\end{lemm}	

From the above Lemma,

\beq
| \|\tilde{X}v\|_2^2 - Tr(\Gamma) | \leq 4 \max\limits_{T \subseteq [1,...n]} |R_T(z)|
\eeq

Therefore we want to compute the probability of the following event:

\beq
P \left \{ \max\limits_{v \in N_{\epsilon}(A), T \subseteq [1,...,n]}   |R_T(z)| > \frac{t}{8} \right \} \leq N \left ( A, \frac{1}{4} \right) \cdot 2^n \cdot \max\limits_{v \in N_{\epsilon}(A), T \subseteq [1,...,n]} P \left \{ |R_T(z)| > \frac{t}{8} \right \}
\eeq

The r.h.s follows from a union bounding argument.

To estimate the probability, we fix a vector $v \in N_{\epsilon}(A)$ and a subset $T \subseteq [1,...n]$ and we condition on a realization of random variables $(Z_k)_{k \in T^c}$. Therefore, we express

\beq
R_T(z) = \sum_{j \in T} Z_j \langle \Gamma_j^{1/2}, b \rangle , \text{ where } b = \sum_{k \in T^c} Z_k\Gamma_k^{1/2}
\eeq

Under this conditioning $b$ is a fixed vector, so $R_T(z)$ is a sum of independent random variables. Moreover,

\beq
\|b\|_2 \leq \|\Gamma^{1/2}\|_2 \|Z\|_2 = \|\Gamma^{1/2}\|_2 \|Xv\|_2 \leq \sqrt{\Lambda_{\max}(\Gamma)}c \sqrt{n}
\eeq

The inequality above follows from our results for the isotropic sub-Gaussian design scenario. It can be proved using the same arguments,

\beq
\|Z\|_2 = \|Xv\|_2 \leq \sqrt{n} + \eta_0 w(A) + \tau \leq c \sqrt{n}
\eeq

For a large enough c the above result is almost always satisfied.
Under these conditions $\sum_{j \in T} Z_j \langle \Gamma_j^{1/2}, b \rangle$ is a sum of independent sub-Gaussian random variables which in turn is a sub-Gaussian variable with sub-Gaussian norm

%\beq
%\|R_T(z)\|_{\psi_2} \leq c_2(\sum_{j \in T} \langle \Gamma_j^{1/2}, b \rangle ^2 \|Z_j\|_{\psi_2}^2)^{1/2} \leq c_2(\|\Gamma_j^{1/2}\|_2^2 %\|b\|_2^2 \sum_{j \in T} \|Z_j\|_{\psi_2}^2)^{1/2} \leq c_3 \Lambda_{\max}(\Gamma)K^2
%\eeq

\beq
\vertiii{R_T(z)}_{\psi_2} \leq K
\eeq

and

\beq
\sum_{j \in T} \langle \Gamma_j^{1/2}, b \rangle \leq \|\Gamma_j\|_2\|b\|_2 \leq \Lambda_{\max}(\Gamma) c \sqrt{n}
\eeq

Denoting the conditional probability by $P_T = P( \cdot | (Z_k)_{k \in T^c})$ and the expectation with respect to $(A_k)_{k \in T^c}$ by $E_{T^c}$, we obtain

\begin{align*}
P \left \{ |R_T(z)| > \frac{t}{8} \right \} &\leq E_{T^c} P_T \left \{ |R_T(z)| > \frac{t}{8} \right \} \\
											&\leq 2 \exp \left [ -c_4 \left ( \frac{t/8}{K \Lambda_{\max}(\Gamma) \sqrt{n}}  \right )^2 \right ] \\
											&\leq 2 \exp \left [ - c_5 \left ( \frac{\delta Tr(\Gamma)}{K \Lambda_{\max}(\Gamma) \sqrt{n}}  \right )^2 \right ]
\end{align*}

Substituting $\delta = \frac{\eta_0 w(A) \Lambda_{\max}(\Gamma)}{\sqrt{Tr(\Gamma)}} + \frac{\tau}{\sqrt{Tr(\Gamma)}}$ and by the earlier argument we get

%\begin{align*}
%P &\left \{ \max\limits_{v \in N_{\epsilon}(A), T \subseteq [1,.,n]}   |R_T(z)| > \frac{t}{8} \right \} \\
%&\leq \exp(c_1 w^2(A)) \exp(n~ln~2) \exp \left [ - c_5 \left ( \frac{\eta_0^2 w^2(A) Tr(\Gamma)}{K^2 n } + \frac{\tau^2 Tr(\Gamma)}{K^2 %\Lambda_{\max}^2(\Gamma) n } + \frac{Tr^2(\Gamma)}{16 K^2 \Lambda_{\max}^2(\Gamma) n} \right ) \right ] \\
%&\leq \exp \left [ - w^2(A) \left ( c_5 \frac{\eta_0^2 Tr(\Gamma)}{K^2 n} - c_1 \right ) \right ] \exp \left [ - \frac{c_5 Tr^2(\Gamma)}{16 %K^2 \Lambda_{\max}^2(\Gamma) n} + n~ln~2 \right ] \exp \left [ - \frac{c_5 \tau^2 Tr(\Gamma)}{K^2 \Lambda_{\max}^2(\Gamma)n} \right ]
%\end{align*}

\begin{align*}
P &\left \{ \max\limits_{v \in N_{\epsilon}(A), T \subseteq [1,.,n]}   |R_T(z)| > \frac{t}{8} \right \} \\
&\leq \exp(c_1 w^2(A)) \exp(n~ln~2) \exp \left [ - c_5 \left ( \frac{\eta_0^2 w^2(A) Tr(\Gamma)}{K^2 n } + \frac{\tau^2 Tr(\Gamma)}{K^2 \Lambda_{\max}^2(\Gamma) n } \right ) \right ] \\
&\leq \exp \left [ - w^2(A) \left ( c_5 \frac{\eta_0^2 Tr(\Gamma)}{K^2 n} - c_1 \right ) + n~ln~2 \right ] \exp \left [ - \frac{c_5 \tau^2 Tr(\Gamma)}{K^2 \Lambda_{\max}^2(\Gamma)n} \right ]
\end{align*}

Choosing $\eta_0 > \sqrt{\frac{c_1 K^2 n}{c_5 Tr(\Gamma)} + \frac{n^2 K^2 ln~n}{c_5w^2(A) Tr(\Gamma)}}$ and $\eta_1 = \frac{c_5 Tr(\Gamma)}{K^2 \Lambda_{\max}^2(\Gamma) n}$ completes the proof \qed

\section{Generalized Linear Models: Restricted Strong Convexity}
\input{supp-glm}

\newpage

%% NEEDS WORK
\bibliographystyle{plain}
\bibliography{supp_norm_ref}

\end{document}
